# Supplementary material for: Sample-Efficient Constrained Reinforcement Learning with General Parameterization
Source: arXiv:2405.10624 source file (2024-10-31)
Supplement: Supplementary file 1 [file lemma4.tex]

\section{Proof of Lemma \ref{lemma_4}}

\begin{proof}
    Recall from Lemma \ref{lemma_2}(b) that $J_{\mathrm{L}, \rho}(\cdot, \lambda)$ is $L(1+\lambda)$-smooth. Therefore,
    \begin{align}
        \begin{split}
            &J_{\mathrm{L}, \rho}(\theta_{k+1},\lambda_k)\geq J_{\mathrm{L}}(\theta_k,\lambda_k)+\left<\nabla_{\theta} J_{\mathrm{L}, \rho}(\theta_k,\lambda_k),\theta_{k+1}-\theta_k\right>-\frac{L(1+\lambda_k)}{2}\Vert\theta_{k+1}-\theta_k\Vert^2\\
            &\overset{(a)} =J_{\mathrm{L}, \rho}(\theta_k,\lambda_k) + \eta \nabla_{\theta} J_{\mathrm{L}, \rho}(\theta_k,\lambda_k)^T \omega_k - \frac{L(1+\lambda_k) \eta^2}{2} \Vert\omega_k\Vert^2 \\
            &= J_{\mathrm{L}, \rho}(\theta_k,\lambda_k) + \eta\langle \nabla_{\theta} J_{\mathrm{L}, \rho}(\theta_k,\lambda_k), \omega_k^*\rangle + \eta\langle \nabla_{\theta} J_{\mathrm{L}, \rho}(\theta_k,\lambda_k), \omega_k-\omega_k^*\rangle \\
            &\hspace{2.3cm}- \frac{L(1+\lambda_k) \eta^2}{2}\Vert\omega_k-\omega_k^*+\omega_k^*\Vert^2\\
            &\overset{}\geq J_{\mathrm{L}, \rho}(\theta_k,\lambda_k) + \eta\langle \nabla_{\theta} J_{\mathrm{L}, \rho}(\theta_k,\lambda_k), F_{\rho}(\theta_k)^{\dagger}\nabla_{\theta}J_{\mathrm{L},\rho}(\theta_k, \lambda_k)\rangle + \eta\langle \nabla_{\theta} J_{\mathrm{L}, \rho}(\theta_k,\lambda_k), \omega_k-\omega_k^*\rangle\\
            &\hspace{2.3cm}- L(1+\lambda_k)\eta^2\Vert \omega_k - \omega_k^* \Vert^2-L(1+\lambda_k)\eta^2\Vert\omega_k^*\Vert^2\\
            &\overset{(b)}{\geq} J_{\mathrm{L}, \rho}(\theta_k,\lambda_k) + \dfrac{\eta}{G^2}\Vert\nabla_{\theta}J_{\mathrm{L}, \rho}(\theta_k, \lambda_k)\Vert^2 + \eta\langle \nabla_{\theta} J_{\mathrm{L}, \rho}(\theta_k,\lambda_k), \omega_k-\omega_k^*\rangle\\
            &\hspace{2.3cm}- L(1+\lambda_k)\eta^2\Vert \omega_k - \omega_k^*\Vert^2 - L(1+\lambda_k)\eta^2 \Vert F_{\rho}(\theta_k)^{\dagger}\nabla_{\theta}J_{\mathrm{L}, \rho}(\theta_k, \lambda_k)\Vert^2\\
            &\overset{(c)}{\geq} J_{\mathrm{L}, \rho}(\theta_k,\lambda_k) + \left(\dfrac{\eta}{2G^2}-\dfrac{L(1+\lambda_k)\eta^2}{\mu_F^2}\right)\Vert\nabla_{\theta}J_{\mathrm{L}, \rho}(\theta_k, \lambda_k)\Vert^2 \\
            &+ \dfrac{\eta}{2G^2}\underbrace{\left[\Vert\nabla_{\theta}J_{\mathrm{L}, \rho}(\theta_k, \lambda_k)\Vert^2 + 2G^2 \langle \nabla_{\theta} J_{\mathrm{L}, \rho}(\theta_k,\lambda_k), \omega_k-\omega_k^*\rangle + G^4\Vert\omega_k-\omega_k^*\Vert^2 \right]}_{=\left\Vert\nabla_{\theta}J_{\mathrm{L}, \rho}(\theta_k, \lambda_k)+G^2(\omega_k-\omega_k^*)\right\Vert^2\geq 0}\\
            &-\left(L(1+\lambda_k)\eta^2+\dfrac{\eta G^2}{2}\right)\Vert\omega_k-\omega_k^*\Vert^2\\
            & \geq J_{\mathrm{L}, \rho}(\theta_k,\lambda_k) + \left(\dfrac{\eta}{2G^2}-\dfrac{L(1+\lambda_k)\eta^2}{\mu_F^2}\right)\Vert\nabla_{\theta}J_{\mathrm{L}, \rho}(\theta_k, \lambda_k)\Vert^2\\
            &\hspace{2.3cm}-\left(L(1+\lambda_k)\eta^2+\dfrac{\eta G^2}{2}\right)\Vert\omega_k-\omega_k^*\Vert^2
        \end{split}
    \end{align}	
    where (a) follows from the update equation $\theta_{k+1}=\theta_k+\eta\omega_k$ and (b), (c) utilize Assumption \ref{ass_score} and \ref{ass_fisher} respectively. Adding $J_{\mathrm{L}, \rho}(\theta_{k+1}, \lambda_{k+1})$ on both sides of the above inequality, we obtain the following.
    \begin{align}
        \label{eq_34}
        \begin{split}
            &J_{\mathrm{L}, \rho}(\theta_{k+1}, \lambda_{k+1}) -J_{\mathrm{L}, \rho}(\theta_{k}, \lambda_{k})\geq J_{\mathrm{L}, \rho}(\theta_{k+1}, \lambda_{k+1}) - J_{\mathrm{L}, \rho}(\theta_{k+1}, \lambda_{k}) \\
            &+ \left(\frac{\eta}{2G^2}-\dfrac{L(1+\lambda_k)\eta^2}{\mu_F^2}\right) \Vert\nabla_{\theta} J_{\mathrm{L}, \rho}(\theta_k,\lambda_k)\Vert^2 - \left(\frac{\eta G^2}{2}+L(1+\lambda_k)\eta^2\right) \Vert \omega_k - \omega^*_k\Vert^2
        \end{split}
    \end{align}
    Observe that,
    \begin{align}
        \label{eq_35}
        \begin{split}
            J_{\mathrm{L}, \rho}(\theta_{k+1}, \lambda_{k+1}) - J_{\mathrm{L}, \rho}(\theta_{k+1}, \lambda_{k}) &= (\lambda_{k+1}-\lambda_k)J_{c, \rho}(\theta_{k+1})\\
            &\overset{(a)}{\geq} -\dfrac{1}{1-\gamma}|\lambda_{k+1}-\lambda_k| \overset{(b)}{\geq} -\dfrac{\zeta}{1-\gamma}\left|\hat{J}_{c, \rho}(\theta_k)\right|
        \end{split}
    \end{align}
    where (a) utilizes the fact that $|J_{c, \rho}(\theta_{k+1})|\leq 1/(1-\gamma)$ whereas (b) results from \eqref{eq:lambda_update} and contractive property of the projection operator $\mathcal{P}_{\Lambda}$. Combining \eqref{eq_34} and \eqref{eq_35}, and using $\lambda_k\leq \lambda_{\max}$, one obtains,
    \begin{align}
        \begin{split}
            &J_{\mathrm{L}, \rho}(\theta_{k+1}, \lambda_{k+1}) -J_{\mathrm{L}, \rho}(\theta_{k}, \lambda_{k})\geq -\dfrac{\zeta}{1-\gamma}\left|\hat{J}_{c, \rho}(\theta_k)\right|\\
            &+ \left(\frac{\eta}{2G^2}-\dfrac{L(1+\lambda_{\max})}{\mu_F^2}\eta^2\right) \Vert\nabla_{\theta} J_{\mathrm{L}, \rho}(\theta_k,\lambda_k)\Vert^2 - \left(\frac{\eta G^2}{2}+L(1+\lambda_{\max})\eta^2\right) \Vert \omega_k- \omega^*_k\Vert^2
        \end{split}
    \end{align}
    Choosing $\eta = \frac{\mu_F^2}{4G^2L(1+\lambda_{\max})}$, and taking a sum over $k\in \{0, \cdots, K-1\}$, we arrive at,
    \begin{align}
        \begin{split}
            &\dfrac{\mu_F^2}{16G^4L(1+\lambda_{\max})}\left(\dfrac{1}{K}\sum_{k=0}^{K-1}\Vert\nabla_{\theta} J_{\mathrm{L}, \rho}(\theta_k, \lambda_k)\Vert^2\right)\leq \dfrac{\zeta}{1-\gamma}\left(\dfrac{1}{K}\sum_{k=0}^{K-1}\left|\hat{J}_{c, \rho}(\theta_k)\right|\right) \\
            &+\dfrac{1}{L(1+\lambda_{\max})}\left(\dfrac{\mu_F^2}{8}+\dfrac{\mu_F^4}{16G^4}\right)\left(\dfrac{1}{K}\sum_{k=0}^{K-1}\Vert\omega_k-\omega_k^*\Vert^2\right) + \dfrac{J_{\mathrm{L}, \rho}(\theta_{K}, \lambda_K)-J_{\mathrm{L}, \rho}(\theta_0, \lambda_0)}{K}
        \end{split}
    \end{align}
    Note that $|J_{\mathrm{L}, \rho}(\theta_{K}, \lambda_K)-J_{\mathrm{L}, \rho}(\theta_0, \lambda_0)|\leq 2(1+\lambda_{\max})/(1-\gamma)$. Moreover, following the sampling procedure described in Algorithm \ref{algo_sampling}, we deduce, $\mathbf{E}|\hat{J}_{c,\rho}(\theta_k)|\leq \sum_{t=0}^{\infty} (1-\gamma)(t+1)\gamma^t = 1/(1-\gamma)$. This leads us to the following.
    \begin{align}
        \begin{split}
             \dfrac{1}{K}\sum_{k=0}^{K-1}\mathbf{E}\Vert\nabla_{\theta} J_{\mathrm{L}, \rho}(\theta_k, \lambda_k)\Vert^2 &\leq (2G^4+\mu_F^2)\left(\dfrac{1}{K}\sum_{k=0}^{K-1}\mathbf{E}\Vert\omega_k-\omega_k^*\Vert^2\right)\\
             &+ \left(\dfrac{32G^4L(1+\lambda_{\max})^2}{\mu_F^2(1-\gamma)}\right)\dfrac{1}{K}+ \left(\dfrac{16G^4L(1+\lambda_{\max})}{\mu_F^2(1-\gamma)^2}\right)\zeta
        \end{split}
    \end{align}
    This completes the proof.
\end{proof}
